# Supplementary material for: Cell assembly dynamics of sparsely-connected inhibitory networks: a simple model for the collective activity of striatal projection neurons
Source: arXiv:1511.06920 ancillary file (2015-11-21)
Supplement: Supplementary file 1 [file SupportingInformation.pdf]

# Supporting Information
# Cell Assembly Dynamics of Sparsely-connected Inhibitory Networks: a Simple Model for the Collective Activity of Striatal Projection Neurons

David Angulo-Garcia*
*CNR - Consiglio Nazionale delle Ricerche - Istituto dei Sistemi Complessi, via Madonna del Piano 10, I-50019 Sesto Fiorentino, Italy*

Joshua D. Berke†
*Department of Psychology, University of Michigan, Ann Arbor, 530 Church St., Ann Arbor, MI 48104, USA*

Alessandro Torcini‡
*Aix-Marseille Université, Inserm, INMED UMR 901 and Institut de Neurosciences des Systèmes UMR 1106, 13005, Marseille, France*
*Aix-Marseille Université, Université de Toulon, CNRS, CPT, UMR 7332, 13288 Marseille, France*
*CNR - Consiglio Nazionale delle Ricerche - Istituto dei Sistemi Complessi, via Madonna del Piano 10, I-50019 Sesto Fiorentino, Italy and*
*INFN Sez. Firenze, via Sansone, 1 - I-50019 Sesto Fiorentino, Italy*

* david.angulo@fi.isc.cnr.it
† jdberke@umich.edu
‡ alessandro.torcini@cnr.it

## TEXT S1

### Active and silent Neurons

We define a neuron as active, if it emits more than $S_\Theta$ spikes within the system evolution, which we typically take as the time taken for the network to evolve through to $10^7$ spikes. In particular, in Fig. S 1 (a) and (b) we report the fraction of active neurons $n^*$ versus the synaptic strength for two parameter settings and for several values of the considered threshold, namely $0 \leq S_\Theta \leq 100$. In practice, we observe that neither the minimal value of $n^*$ nor the value for which the minimum is reached, appears to strongly depend on the chosen threshold, thus demonstrating the robustness of the results that we present through the article.

### Mechanisms for the resurgence of silent neurons

In what follows we report the neuronal distributions of the average inter-spike intervals $\overline{ISI}$, of the corresponding $CV$, of the associated average effective synaptic input $\overline{W}_i \equiv I_i - g\overline{E}_i$ and standard deviation $\sigma(W_i)$. In particular, we consider these distributions for two different stimuli dispersion (namely, $\Delta V = 5$ mV and 1mV) as well as for two synaptic strengths (namely, $g \simeq g_{min}$ and $g >> g_{min}$).

For $\Delta V = 5$ mV ($\Delta V = 1$ mV) we examine two synaptic strengths, one in proximity of the minimum $g_{min}$ of $n^*$, where almost 50 % of neurons are active, and one for which almost all the neurons are active again, namely $g = 4$ and 10 ($g = 1$ and 4). Let us first consider the distribution of the average $\overline{ISI}$ of the single cell reported in Fig S 2(a) and (d). At small $g$ the distributions reveal a clear peak at some low $\overline{ISI}$ plus a long tail. In correspondence of this coupling the distribution of $CV$ is clearly bimodal as shown in Fig S 2(b) and (e) with peaks around zero and one, thus indicating that the neurons associated to the peak in $P(\overline{ISI})$ are firing in a regular fashion, while the neurons in the tail of $P(\overline{ISI})$ contributes to the second peak in $P(CV)$ around $CV \simeq 1$. Furthermore, by examining the distributions of the average effective input $\overline{W}_i$ perceived by each single cell, the PDF for $g \simeq g_{min}$ has a peak in proximity the threshold value $V_{th}$.

We can conclude that the neurons contributing to the main peaks in $P(\overline{ISI})$ and $P(CV)$ for $g \simeq g_{min}$ are the *winners*, which fire faster than the others and almost periodically, thus suggesting that they are not particularly influenced by the other neurons in the network. Moreover, they correspond to the neurons which are on average above threshold, as shown in Fig. S 2(c) and (f). The neurons contributing to the second maximum in $P(CV)$ and to the tail of $P(\overline{ISI})$ are instead slow neurons whose activity is strongly depressed by the winners and they are neurons around, or just below threshold, in Fig. S 2(c) and (f).

As one can appreciate from Fig. S 2(a) and (d) the $P(\overline{ISI})$ is completely modified at large $g$. In such a case, a broad peak is present extending over two orders of magnitude. In this regime the majority of the cells are on average below-threshold, as it can be appreciated by the corresponding $P(\overline{W}_i)$, reported in Fig. S 2(c) and (f) as red empty squares, which reveal an almost Gaussian shape centered well below threshold. Therefore we are now in a situation where all neurons are active, but the majority are activated due to the fluctuations in the input and they are no more tonically firing. The fact that now the activity is mostly fluctuation driven, is reflected also in the $CV$ distributions, which are now centered well above one.

The reported results clearly show that for wider dispersion of the $I_i$, as measured by $\Delta V$, a greater lateral inhibition is required to observe similar effects.

As explained in the sub-section *The role of lateral inhibition* in the article and as evident from Fig. S 3(a) and (b), by increasing the synaptic strength not only the average effective input $\langle \bar{W} \rangle$ but also the fluctuations on the effective input $\langle \sigma(W) \rangle$ increases. In particular, the transition among the two dynamical regimes, occurring at $g = g_{min}$, is due to a passage from a state where a part of the neurons identified as the *winners* were mean-driven and were able to depress all the other neurons, to a state at $g >> g_{min}$ where almost all neurons are fluctuation driven and all the neurons contribute to the network activity. The transition occurs because at $g < g_{min}$ the fluctuations of the effective input currents $W_i$ are small and insufficient to drive the losers towards the firing threshold (as shown in the insets of Fig. S2 (c) and (f)). At $g \simeq g_{min}$ the amplitude of fluctuations begin to be sufficient to lead some loser to rise again above threshold and to contribute to the number of active neurons. This will also contribute to moderate the winners activity. For $g >> g_{min}$ the fluctuations of $W_i$ are sufficient to restore all losers to the firing activity and at the same time no clear distinction among losers and winners can be done. The transition is due to the fact that not only the inhibitory action is proportional to the synaptic strength, but also the fluctuation amplitude increases linearly with $g$, at least for $g > g_{min}$ (as shown in Figs. S3(a) and (b)).

**Linear stability analysis**

One of the questions that we would like to address is whether the existence of a bursting correlated activity is related to linear stability properties of the network or not. To characterize these properties, we calculate the maximal Lyapunov exponent (LE) $\lambda$ for the parameters examined in the text. In order to compute the LE we derive from Eq. (3) (main text) its linearization, which describes the evolution of infinitesimal perturbations in the reference orbits, this reads as:

$$\begin{aligned}\delta E_i(n+1) &= \mathrm{e}^{-\alpha\tau(n)}\left[\delta E_i(n) + \tau(n)\delta P_i(n)\right] \\ &\quad - \mathrm{e}^{-\alpha\tau(n)}\left[\alpha E_i(n) + (\alpha\tau(n) - 1)P_i(n)\right]\delta\tau(n)\,, \end{aligned} \tag{S1a}$$

$$\delta P_i(n+1) = \mathrm{e}^{-\alpha\tau(n)}\left[\delta P_i(n) - \alpha P_i(n)\delta\tau(n)\right]\,, \tag{S1b}$$

$$\begin{aligned}\delta v_i(n+1) &= \mathrm{e}^{-\tau(n)}\left[\delta v_i(n) + (a - v_i(n))\delta\tau(n)\right] + g\delta H_i(n) \\ i &= 1, \dots, N \quad ; \quad \delta v_m(n+1) \equiv 0\,. \end{aligned} \tag{S1c}$$

The boundary condition $\delta v_m(n+1) \equiv 0$ is a consequence of the event driven evolution. The expression of $\delta\tau(n)$ can be computed by differentiating Eqs. (4) and (5) (in main text), namely

$$\delta\tau(n) = \tau_v \delta v_m(n) + \tau_E \delta E_m(n) + \tau_P \delta P_m(n)\,, \tag{S2}$$

where

$$\tau_v := \frac{\partial\tau}{\partial v_m} \quad , \quad \tau_E := \frac{\partial\tau}{\partial E_m} \quad , \quad \tau_P := \frac{\partial\tau}{\partial P_m} \quad . \tag{S3}$$

The maximal LE $\lambda$ is defined as the the average exponential growth rate of the infinitesimal perturbation

$$\delta = (\delta v_1 \dots \delta v_N,\, \delta E_1 \dots \delta E_N,\, \delta P_1 \dots \delta P_N)$$

measured through the equation

$$\lambda = \lim_{t\to\infty} \frac{1}{t} \log \frac{\mid \delta(t) \mid}{\mid \delta_0 \mid} \quad , \tag{S4}$$

where $\delta_0$ is the initial perturbation. The evolution of the perturbation $\delta(t)$ at the following times can be obtained by integrating Eqs. (S1) in the tangent space in parallel with the evolution in the real space and by performing at regular time intervals the rescaling of its amplitude to avoid numerical artifacts, as detailed in [2]. A positive $\lambda$ denotes a chaotic dynamics, a zero maximal LE is associated to a periodic (or quasiperiodic) orbit, and a negative one to a stable fixed point. It is important to stress that, since we are dealing with an event driven map formulation of the dynamics, the zero Lyapunov exponent which is always present for continuous time evolution and associated to the growth rate of a perturbation along the orbit, is automatically discarded. This implies that, if the evolution is stable, either a fixed point or a periodic solution, we measure in both cases a maximal LE $\lambda < 0$.

For a fixed pulse duration $\tau_\alpha = 20$ ms, the behaviour of the maximal LE $\lambda$ as a function of the coupling $g$, for different excitability spreading $\Delta V$, is definitely different. As shown in Fig S4 (a), for $\Delta V = 1$ mV the LE (as expected) is zero for very weakly coupled systems, then it first increases with $g$ and reaches a maximum around $g = 2$ and then it decreases monotonically becoming negative for $g > 5$. For $\Delta V = 5$ mV, the LE is always positive and increases with $g$ saturating at an almost constant value $\lambda \simeq 3.4$ Hz for $g \geq 6$. We are specifically interested in the conditions for which the measure $Q_0$ is maximized, these points are indicated in Fig S4 (a), as one can notice they correspond for both considered $\Delta V$ to positive $\lambda$.

Additionally we have analyzed the behaviour of $\lambda$ as a function of $\tau_\alpha$ by fixing $g$ to the value that maximizes $Q_0$ in the previous analysis. In this case it appears that $\lambda$ increases with $\tau_\alpha$ and becomes definitely negative for sufficiently small $\tau_\alpha$ (as shown in Fig. S4 (b)), in agreement with the results reported in [1, 3]. The cell assembly dynamics of our network resembles that of MSNs for large $\tau_\alpha$, as explained in the text, the point where $Q_0$ is maximal are indicated also in Fig. S4 (b). These evidences seem to suggest that the striatally relevant dynamics correspond to a chaotic regime, but located in proximity of the transition between chaotic and non-chaotic evolution. The same conclusion was already reported for a rate model of the striatum in [6].

However, all this analysis and the one reported in [6] consider only infinitesimal perturbations, while it has been clearly demonstrated that for inhibitory networks finite perturbations play a fundamental role as shown in [1, 3, 4, 7]. In particular our model, even for $\lambda < 0$, can display erratic evolution almost indistinguishable from chaos due to the so-called Stable Chaos mechanism [1, 5]. This leads us to conclude that the usual Lyapunov exponent is unable to capture the degree of erratic motion present in these systems, due to the possible amplification of finite amplitude perturbations.

### State Transition Matrices for different regimes

In the main text we have just reported the averaged State Transition Matrix (STM) corresponding to the consecutive presentation of two stimuli for parameters obtained by maximizing $Q_0$. Here we want to show how the STM is modified by considering $\tau_\alpha = 20$ ms, for which $Q_0$ is maximal, and for a smaller pulse duration, namely $\tau_\alpha = 2$ ms, for which the evolution of the network is seemingly Poissonian. The upper panel of Fig S6 show another realization of the network obtained for the same parameters of Fig. 5 (in main text). The lower panels correspond to $\tau_\alpha = 2$ms. The raster plots clearly show that for $\tau_\alpha = 20$ ms the network exhibits a clear patterned activity with frequent switch from an activated assembly to another, furthermore there is a low correlation between the network activities in presence of the two different stimuli. As shown in Fig S 6 (b,c). For $\tau_\alpha = 2$ ms the system presents much less variability. While it is still capable of discriminating between two different stimuli, now the system fails in revealing a clear assembly switching during the presentation of a single stimulus (see lower panels of Fig. S 6).

### Synchronized Event Transition Matrices and number of coactive cells for different network realizations

We present two different realizations of the numerical experiment performed in the sub-section *Physiological relevance for biological networks under different experimental conditions*. The difference between the realizations lies on the random connectivity matrix $C_{ij}$, which is generated at each realization with the same connection probability. The results are presented in Fig. S 8. More precisely, in Figs. S 8 (a) and S 8 (e) are reported the SETMs for maximal $Q_0$ ($g = 8$ for the chosen parameters). These are characterized by a large variability in their elements when compared with the corresponding SETMs obtained for decreased inhibition (namely, $g = 1$), shown in Figs. S 8 (c) and S 8 (g), is always smaller. The difference between the two regimes is also evidenced in the number of coactive cells: at maximal $Q_0$ each state is well defined, as illustrated in Figs. S 8 (b) and S 8 (f). Since diagonal elements (representing the number of neurons active in a given state) present larger bars compared with the off-diagonal ones (representing the overlap between two different states) Instead, in the set-up with $g = 1$ the states are hardly distinguishable, diagonal and off-diagonal bars have similar heights (as shown in Figs. S 8d) and S 8h))

---


[1] Angulo-Garcia, D. and Torcini, A. (2014). Stable chaos in fluctuation driven neural circuits. *Chaos, Solitons & Fractals*, 69(0):233 – 245.

[2] Benettin, G., Galgani, L., Giorgilli, A., and Strelcyn, J.-M. (1980). Lyapunov characteristic exponents for smooth dynamical systems and for hamiltonian systems; a method for computing all of them. part 1: Theory. *Meccanica*, 15(1):9–20.

[3] Jahnke, S., Memmesheimer, R.-M., and Timme, M. (2009). How chaotic is the balanced state? *Front. Comp. Neurosci.*, 3(13).

[4] Monteforte, M. and Wolf, F. (2012). Dynamic flux tubes form reservoirs of stability in neuronal circuits. *Phys. Rev. X*, 2:041007.

[5] Politi, A. and Torcini, A. (2010). Stable chaos. In *Nonlinear Dynamics and Chaos: Advances and Perspectives*, pages 103–129. Springer.

[6] Ponzi, A. and Wickens, J. (2012). Input dependent cell assembly dynamics in a model of the striatal medium spiny neuron network. *Frontiers in systems neuroscience*, 6.

[7] Zillmer, R., Livi, R., Politi, A., and Torcini, A. (2006). Desynchronization in diluted neural networks. *Phys. Rev. E*, 74(3):036203.

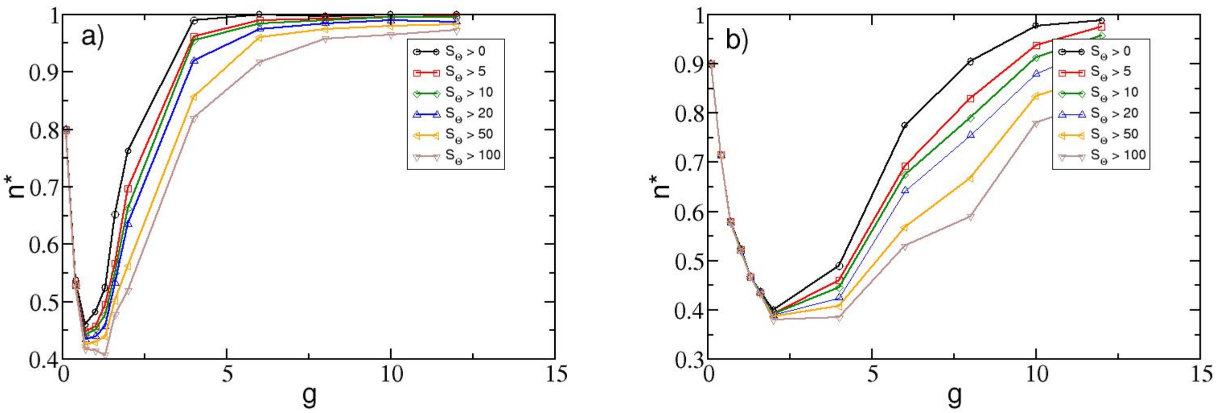


Fig S 1. **Dependence of the value $n*$ on the chosen threshold $S_\Theta$** Fraction of active neurons $n^*$ vs the synaptic strength, for several threshold definitions. A neuron is considered active if it emits at least $S_\Theta$-times during the observation time. Panel a) for $\Delta V = 1$ mV and b) for $\Delta V = 5$ mV. The system is left to evolve during $10^7$ spikes, after discarding $10^5$ spike events of transient. Other parameters used in the simulation: $K = 20$, $N = 400$ and $\tau_\alpha = 20$ms.

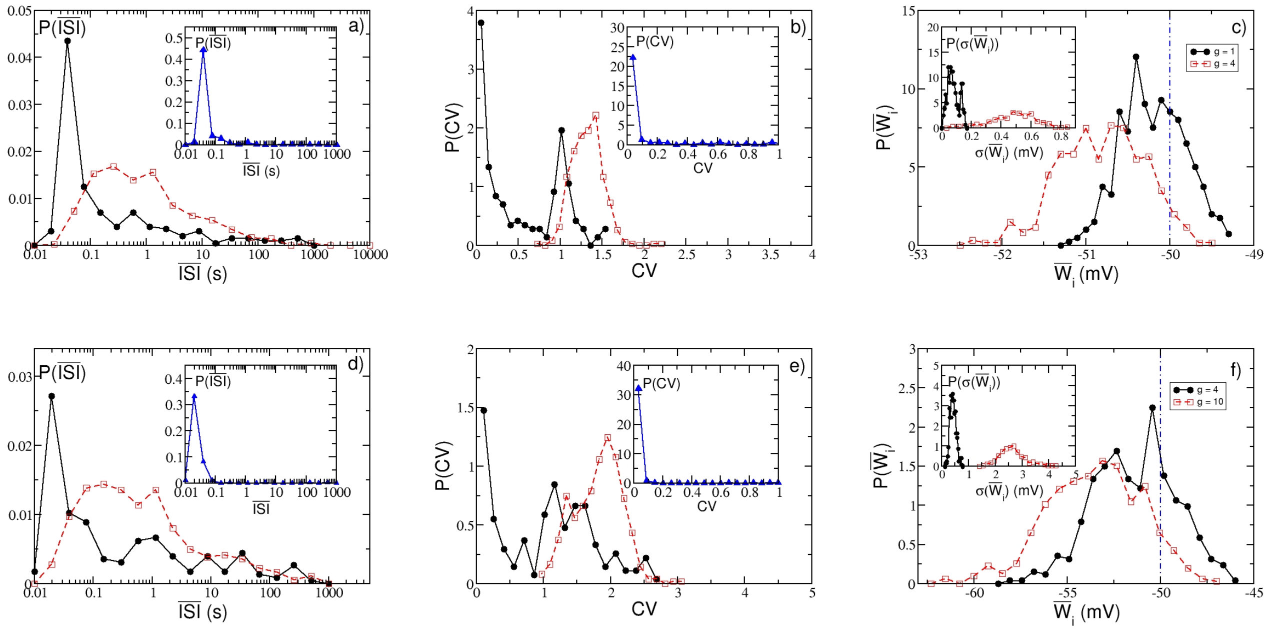


Fig S 2. **Neuronal statistics.** Neuronal distributions of the average $\overline{ISI}$ (a,d), of the coefficient of variation $CV$ (b,e) and of the average effective synaptic input $\overline{W}_i$ (c,f). The data in the first row are for $\Delta V = 1$ mV and in the second one for $\Delta V = 5$ mV. For $\Delta V = 1$ mV ($\Delta V = 5$ mV) black solid line with filled circles correspond to $g = 1$ ($g = 4$) and red dashed lines with open squares to $g = 4$ ($g = 10$). Insets of (a,d) and (c,f), same as the main figure in a lower $g$ regime: $g = 0.4$ ($g = 1$) for $\Delta V = 1$ mV ($\Delta V = 5$ mV). The system is left to evolve during $10^7$ spikes, after discarding $10^5$ spike events. Other parameters used in the simulation: $K = 20$, $N = 400$ and $\tau_\alpha = 20$ ms.

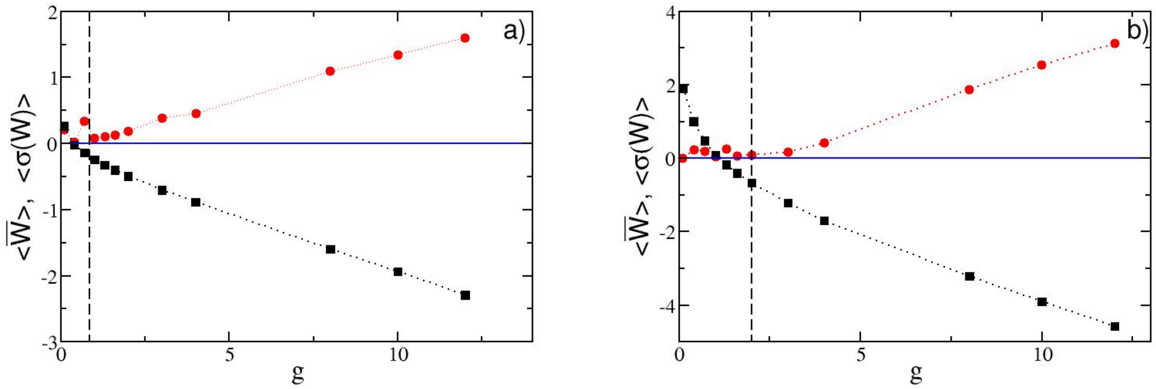


Fig S 3. **Effective input currents and fluctuations.** Effective input currents $\langle\overline{W}\rangle$ (black filled squares) and the corresponding standard deviation $\langle\sigma(W)\rangle$ (red filled circles) averaged over all the neurons in the network for $\Delta V = 1$ mV (a) and $\Delta V = 5$ mV (b). The effective currents are shifted by $V_{th}$: negative (positive) values correspond to neurons on average below (above) threshold. The dashed vertical lines indicated the position of $g_{min}$. The system is left to evolve for $10^7$ spikes, after discarding $10^5$ spike events and the units for $W$ and $\sigma(W)$ are in mV. Other parameters used in the simulation: $K = 20$, $N = 400$ and $\tau_\alpha = 20$ms.

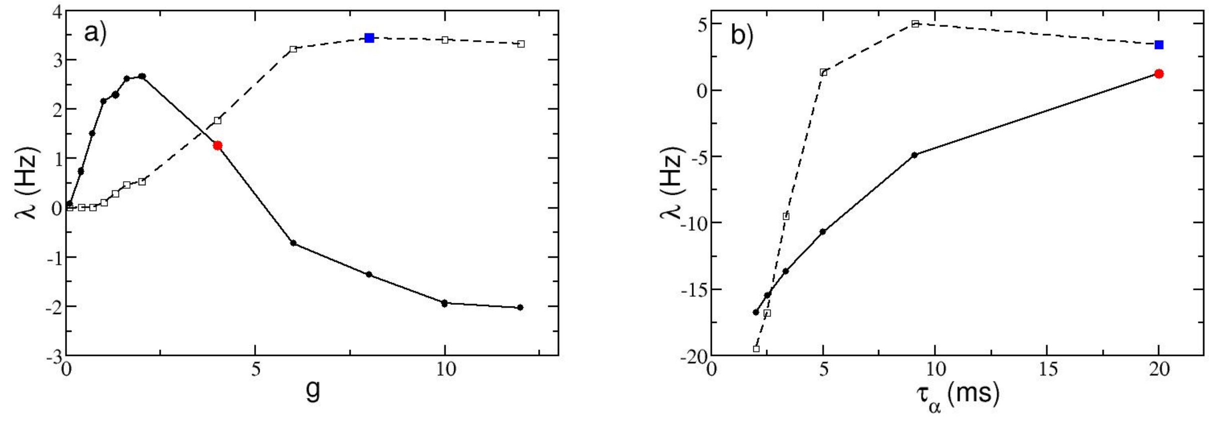


Fig S 4. **Linear stability analysis**. a) Maximal Lyapunov exponent $\lambda$ at a fixed $\tau_\alpha = 20$, as a function of the synaptic strength for $\Delta V = 1$ mV (continuous line, filled circles) and $\Delta V = 5$ mV (dashed line, empty squares). b) Maximal Lyapunov exponent $\lambda$ as a function of the pulse duration $\tau_\alpha$ for the parameters $\{\Delta V, g\} = \{1 \text{ mV}, 4\}$ (continuous line with filled circles) and $\{5 \text{ mV}, 8\}$ (dashed line with empty squares). In both panels, the blue filled square indicates the triad $\{\Delta V, g, \tau_\alpha\} = \{5 \text{ mV}, 8, 20 \text{ ms}\}$, and the red filled circle to $\{\Delta V, g, \tau_\alpha\} = \{1 \text{ mV}, 4, 20 \text{ ms}\}$; these values are associated to the maximum values of $Q_0$ obtained for excitability distributions with fixed width $\Delta V$. The tangent space Eq. (S1) is evolved during a period corresponding to $10^6$ spikes, after discarding a transient of $10^5$ spikes. Other parameters used in the simulation: $K = 20$, $N = 400$.

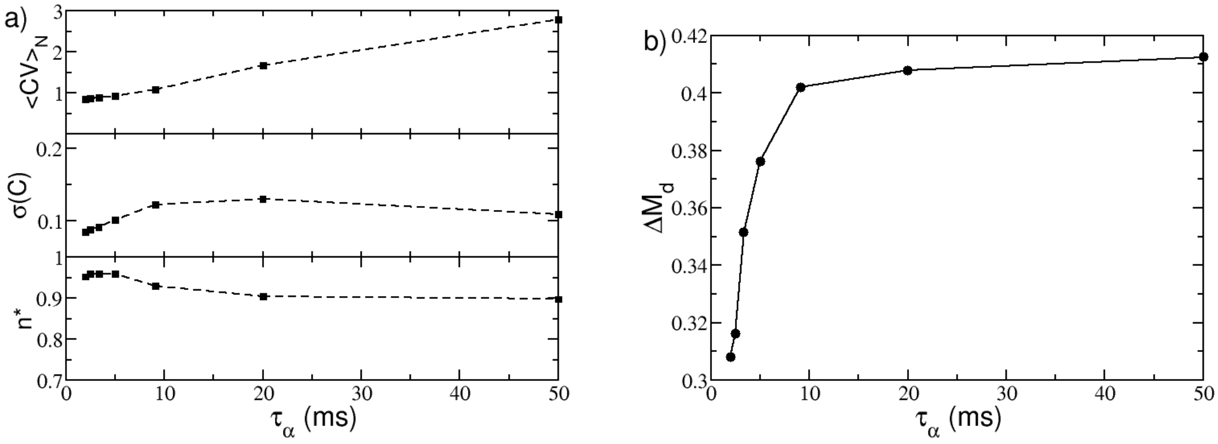


Fig S 5. **Metrics of the structured activity vs synaptic time decay.** a) Metrics entering in the definition of $Q_0$ and their dependence from $\tau_\alpha$. From top to bottom: Averaged coefficient of variation $\langle CV\rangle_N$, standard deviation of the cross-correlation matrix $\sigma(C)$, and the fraction of active neurons $n^*$. b) $\Delta M_d$ as a function of $\tau_\alpha$. The system is left to evolve during $10^7$ spikes, after discarding $10^5$ transient spike events. Parameters here used $\Delta V = 5$ mV, $g = 8$, $K = 20$, $N = 400$.

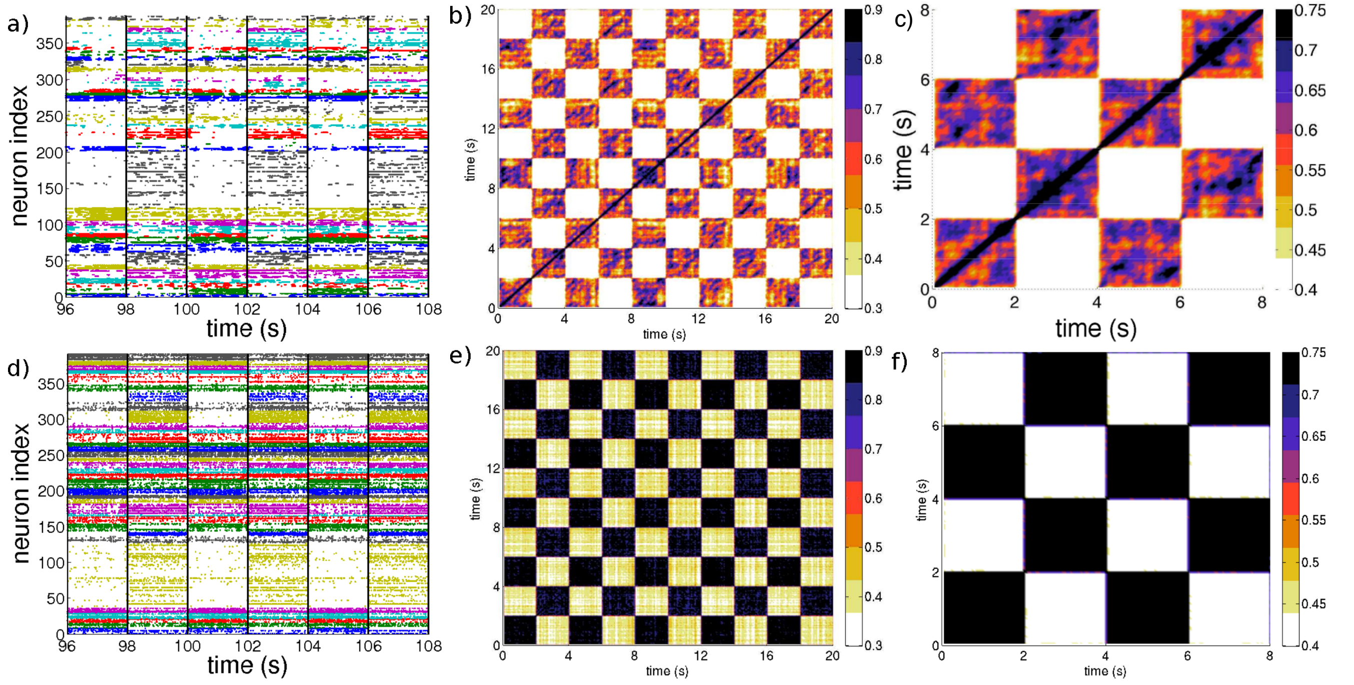


Fig S 6. **Two stimuli presentation.** Upper panel, another realization of the network with the same parameters as chosen in the main text and $\tau_\alpha = 20$ms. Lower panel, network with $\tau_\alpha = 2$ms. From left to right it is depicted the raster plot colored according to the *k-means* algorithm with $k$=25, vertical lines indicates the change of the presented stimulus. In the middle column is reported the state transition matrix calculated over a time span of 20 seconds (the stimulation protocol is repeated 5 times). Rightmost column reports the state transition matrix for a block 4 s $\times$ 4 s averaged over $r = 5$ successive presentations of the inputs.

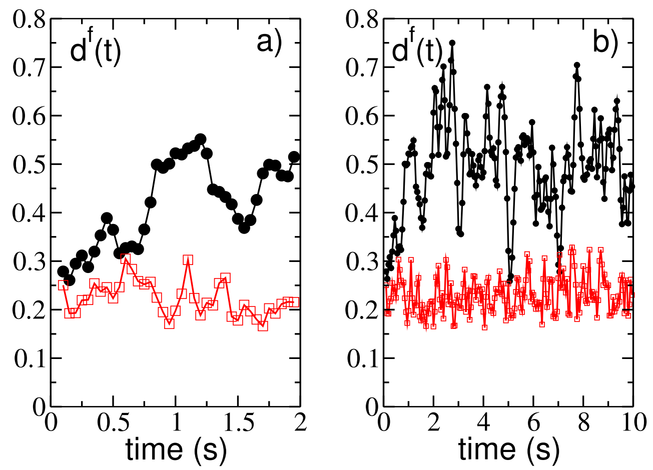


Fig S 7. **Pattern Separation.** Dissimilarity measure in time for an observation window of length a) $T_E = 2$ s and b) $T_E = 10$ s, for two values of $\tau_\alpha$=20 ms (black circles) and $\tau_\alpha$=2 ms (red squares) at a fixed value of $f = 0.2$. It is clearly observed that $\tau_\alpha = 20$ ms more effectively differentiates the similar inputs in both observation windows, as seen by the larger values of dissimilarity respect to the $\tau_\alpha = 2$ms. The initial increase of $d^f(t)$ observable for $\tau_\alpha = 20$ ms in panel (a) is probably due to the fact that the dynamics for this choice of parameters is chaotic as shown in the *Linear stability analysis* sub-section. Therefore the increase can be associated to a transient evolution towards the final attractor. Other parameters used: $\Delta T = 50$ ms, $g = 8$, $N = 400$, $K = 20$.

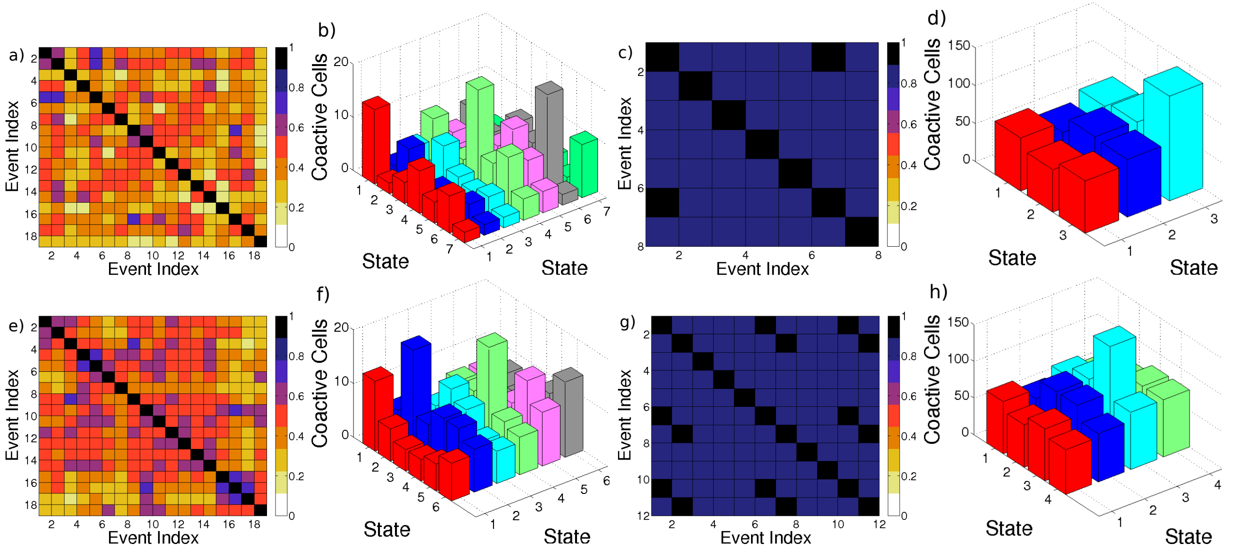


Fig S 8. **Response of the network to an increase in the excitability.** Two different realizations of the numerical experiment reported in the subsection *Physiological relevance for biological networks under different experimental conditions* of the main text. First (third) column reports two realizations of the SETM estimated for $g = 8$ ($g = 1$). Second (fourth) column displays the number of coactive cells in the corresponding cases for $g = 8$ ($g = 1$). The other parameters for the reported simulations are $\Delta V = 5$ mV, $K = 20$, $N = 400$.
